# Supplementary material for: Fair Set Cover
Source: arXiv:2405.11639 source file (2025-04-21)
Supplement: Supplementary file 1 [file proofs.tex]

\section{Initial proofs with other assumptions}
\subsection{Unweighted}
such that $\group(\set_A)=\group_1$, $\group(\set_B)=\group_2$
Let's say we have two demographic groups for sets called $c_1$ and $c_2$. At each iteration, we find a pair of sets $(A, B)$ such that $A \in c_1$ and $B \in c_2$ and the union size $A \cup B$ is as large as possible. We add this pair to our cover and repeat this process for the remaining sets and uncovered points. This will give us a {\bf $\log n$} approximation ratio.

\paragraph{Analysis}
Let's define $S^{\prime}_i$ as the set of points not covered so far at iteration $i$ of our algorithm and $C_i$ as the set of pairs picked so far at iteration $i$. Let's say that the minimum cover $C^*$ has $opt$ number of pairs from the two colors. Let $C^*_i$ be the set of pairs $(A, B)$ from $C^*$ such that at least one of $A$ or $B$ is not picked in $C_i$.

The set $C^*_i$ is a cover for $S^{\prime}_i$. This means that we can cover $S^{\prime}_i$ with $opt$ set pairs. As a result, there is at least one pair $(A, B)$ that satisfies either of the following conditions:
\begin{enumerate}
    \item $A \notin C_i$ and $B \notin C_i$ and $|A \cup B| \geq \frac{|S^{\prime}_i|}{opt}$.
    \item Exactly one of $A$ or $B$ is not in $C_i$, let's say $A$ WLOG, and $|A| \geq \frac{|S^{\prime}_i|}{opt}$.
\end{enumerate}

At the next iteration $i + 1$, we will pick a pair $(C, D)$ with the largest union size. We claim that the size of this union is at least $\frac{|S^{\prime}_i|}{opt}$.

If the $(A, B)$ mentioned above, satisfies first condition, then $|C \cup D| \geq |A \cup B| \geq \frac{|S^{\prime}_i|}{opt}$. Otherwise, if $(A, B)$ satisfies second condition, then $|C \cup D| \geq |A \cup B^\prime|$ where $B^\prime$ can be any set from $C^*_i$ that belongs to the group $c_2$.\footnote{We assumed WLOG that in the pair $(A, B)$, $A$ is in $C^*_i$ but $B$ is not.} As a result, $|C \cup D| \geq |A \cup B^\prime| \geq |A| \geq \frac{|S^{\prime}_i|}{opt}$.

This means $|S^{\prime}_{i + 1}| \leq |S^{\prime}_i| (1 - \frac{1}{opt})$.

\begin{align}
    |S^{\prime}_{i}| &\leq |S^{\prime}_{i - 1}| (1 - \frac{1}{opt}) \\
    &= |S^{\prime}_0| (1 - \frac{1}{opt})^i \\
    &= |X| (1 - \frac{1}{opt})^i \\
    &= n (1 - \frac{1}{opt})^i \\
    &\leq n e^{-\frac{i}{opt}}
\end{align}

Let's say we pick a total of $l$ set pairs in our algorithm. At the last iteration $S_l = \emptyset$. So an upper bound on $l$ would be when $n e^{-\frac{l}{opt}} < 1$.

\begin{align*}
    n e ^ {-\frac{l}{opt}} < 1 \Longleftrightarrow k = O(opt \log n).
\end{align*}

If we have an approximation ratio of $\alpha$ for the \textbf{fair max k cover} problem. Applying this approximation algorithm at each iteration will result in an approximation ratio of $\alpha \log n$ for the \textbf{fair set cover problem}.

\begin{comment}
\subsection{Alternating Algorithm [TO BE REMOVED]}
Let's assume we can cover our set $U$ with the sets belonging to each color $c_j$ with a minimum size of $opt_j$ sets! In this algorithm, we pick a set from color $c_j$ that covers most of the non-covered points so far. In the next step, we do the same with the color $j + 1$ and so on (cyclic iteration on colors).

Let $S^{\prime}_i$ denote the set of points not covered at iteration $i$ of our algorithm. At the next iteration, we are picking a set from color $c_j$ with the largest size on $S^{\prime}_i$. We know that we can cover $S^{\prime}_i$ with at most $opt_i$ sets of $c_j$. So there is a set belonging to color $c_j$ such that it contains more than $\frac{1}{opt_j}$ of $S^{\prime}_i$.

\begin{align*}
    |S^{\prime}_{i+1}| &\leq (1 - \frac{1}{opt_j}) |S^{\prime}_i| \\
    &\leq (1 - \frac{1}{opt_{max}}) |S^{\prime}_i|
\end{align*}

Where $opt_{max}$ is $max\{opt_j | 1 \leq j \leq k\}$. As a result, this algorithm will give a cover with a size at most $O(opt_{max} \log n)$ and the approximation ratio is $O(\frac{opt_{max}}{opt} \log n)$.
\end{comment}

\subsection{Weighted}
In this section, we propose a Greedy Algorithm that gives an $O(L \log(n))$ approximation ratio for Fair Weighted Set Cover. In the following sections, we prove that this is the best approximation ratio one can achieve in polynomial time for this problem.

This is an iterative algorithm. We start from an empty set $X_1$. In each iteration $i$, we add two sets of a pair $(S_{a, i}, S_{b, i})$ to $X_{i}$ to create $X_{i + 1}$, such that $S_{a, i} \in c_1$ and $S_{b, i} \in c_2$ (generalize this to $k$ color case by considering tuples instead of pairs).

After covering all the points, the final $X$ would be the resulting cover. In the iteration $i$, $X_i$ denotes the picked sets before executing this iteration. We also define $Y_i$ as the set of uncovered points before executing this iteration. Let $\optCover$ denote the optimum solution to this problem.

In the iteration $i$, we choose the pair $(S_{a, i}, S_{b, i})$ such that it minimizes the value $\frac{w(S_{a}) + w(S_{b})}{|Y_i \cap (S_{a} \cup S_{b})|} \quad \forall (S_a, S_b): S_a \in c_1, S_b \in c_2$.

\begin{theorem}
    The above algorithm gives us an $O(L \log(n))$ approximation ratio. In other words, $w(X) \leq O(L \log(n)) w(X^*)$.
\end{theorem}

\begin{proof}
    Let $X^*_{paired}$ contain the pairs in the optimum solution. Let $(S_{a, i}, S_{b, i})$ be the pair that we choose in the iteration $i$ by solving the above $\argmin$ equation. In this iteration, the algorithm tries to find the best pair from the set of candidates $\Sets \setminus X_i$.

    From these candidates, some of them are present in the optimum solution $X^* \cap (\Sets \setminus X_i)$. For each set $S_t \in X^* \cap (\Sets \setminus X_i)$, let $p^*(S_t)$ denote the associated pair in the $X^*_{paired}$ that contains this set. For each set $S_t \in X^* \cap (\Sets \setminus X_i)$ define a new function $p(S_t)$ that assigns a pair to a set such that:

    \begin{itemize}
        \item If all the sets inside $p^*(S_t)$ (in case of $k = 2$, the other set) are present in $X^* \cap (\Sets \setminus X_i)$, then $p(S_t) = p^*(S_t)$.
        \item If only $\alpha$ sets of $p^*(S_t)$ are present in $X^* \cap (\Sets \setminus X_i)$, then choose $k - \alpha$ sets arbitrarily from $\Sets \setminus X_i$ each having different color and make a tuple $\gamma$. Then $p(S_t) = \gamma$.
    \end{itemize}

    Note: Based on our assumption in the first sections, we can always find sets of any color inside $X^* \cap (\Sets \setminus X_i)$ as long as we don't cover all the points. It might be the case that a set inside $X^* \cap (\Sets \setminus X_i)$ be present in more than one pair of $p(S_t)$.

    \begin{lemma}
         Let $P = \{p(S_t) | S_t \in X^* \cap (\Sets \setminus X_i)\}$. $\sum_{\gamma \in P} w(\gamma) \leq L w(X^*)$. Where the function $w$ is calculating the sum of weights of sets inside a pair.
    \end{lemma}

    For each pair $\gamma$, let $f(\gamma)$ be the set of sets inside $\gamma$ that are also present in $X^* \cap (\Sets \setminus X_i)$. Based on the definition, we know that $f(\gamma)$ is never empty and $f(\gamma) \subset p^*(S_t)$. Define a function $f^*(\gamma)$ on a pair $\gamma$ that return the pair $\gamma^*$ from $X^*_{paired}$ such that $f(\gamma) \subset \gamma^*$. There is exactly one such pair in $X^*_{paired}$, since the pairs inside $X^*_{paired}$ are disjoint. As a result, the function $f^*$ maps each pair in $P$ to a different pair in $X^*_{paired}$.

    \begin{proof}
        \begin{align}
            \sum_{\gamma \in P} w(\gamma) &= \sum_{\gamma \in P} \sum_{S_t \in \gamma} w(S_t) \\
            &= \sum_{\gamma \in P} (\sum_{S_l \in f(\gamma)} w(S_l) + \sum_{S_q \in \gamma \setminus f(\gamma)} w(S_q))\\
            &\leq \sum_{\gamma \in P} L \sum_{S^*_q \in f^*(\gamma)} w(S^*_q)\\
            &\leq L \sum_{\gamma^* \in X^*_{paired}} w(\gamma^*) = L w(X^*)
        \end{align}
    \end{proof}

    In the iteration $i$, we are picking $(S_{a, i}, S_{b, i})$ such that:
    \begin{align}
    \frac{w(S_{a, i}) + w(S_{b, i})}{|Y_i \cap (S_{a, i} \cup S_{b, i})|} &\leq \frac{w(S_a) + w(S_b)}{|Y_i \cap (S_a \cup S_b)|}, \\
    &\forall S_a, S_b \in \Sets \setminus X_i, \\
    &S_a \in c_1, S_b \in c_2
    \end{align}

    As a result, the following inequality also holds for each pair inside $P$. So, the left-hand side is less than the average sum of weights divided by size on all these pairs:

    \begin{align}
    \label{equ_1}
        \frac{w(S_{a, i} + w(S_{b, i}))}{|Y_i \cap (S_{a, i} \cup S_{b, i})|} &\leq \frac{\sum_{(S^*_a, S^*_b) \in P} w(S^*_a) + w(S^*_b)}{|\bigcup_{(S^*_a, S^*_b) \in P} (S^*_a \cup S^*_b)|} \\
        &\leq \frac{L w(X^*)}{|\bigcup_{(S^*_a, S^*_b) \in P} (S^*_a \cup S^*_b)|}\\
        &\leq \frac{L w(X^*)}{|Y_i|} \label{remain_size}
    \end{align}

    The line ~\ref{remain_size} is because we already know that we can cover all $Y_i$ using the sets inside $X^* \setminus X_i$. 
    
    For each point $\element_j \in \Elements$ let $\Gamma(e_j)$ be the pair that covered this point for the first time while running the Greedy Algorithm and $I(e_j)$ be the iteration number in which this pair is selected.

    \begin{lemma}
    \label{lem_upper}
        Let $X_{paired}$
        \begin{align}
            \sum_{\element_j \in \Elements} \frac{\sum_{S_t \in \Gamma(e_j)} w(S_t)}{|Y_{I(e_j)} \cap (\bigcup_{S_t \in \Gamma(e_j)} S_t)|} = w(\cover).
        \end{align}
        Where $\cover$ is the final cover.
    \end{lemma}

    \begin{proof}
    Let $X_{paired}$ be the pairs inside $\cover$ and for each $p \in X_{paired}$, $\lambda(p)$ be the set of points covered by this pair for the first time. In other words, when picking this pair, all points inside this pair, except $\lambda(p)$, were covered before. For a point $e_j \in \lambda(p)$ we have $|\lambda(p)| = |Y_{I(e_j)} \cap (\bigcup_{S_t \in p} S_t)|$.
    
        \begin{align}
            \sum_{\element_j \in \Elements} \frac{\sum_{S_t \in \Gamma(e_j)} w(S_t)}{|Y_{I(e_j)} \cap (\bigcup_{S_t \in \Gamma(e_j)} S_t)|} &=\\
            &\sum_{p \in X_{paired}} \sum_{e_j \in \lambda(p)} \frac{\sum_{S_t \in \Gamma(e_j)} w(S_t)}{|Y_{I(e_j)} \cap (\bigcup_{S_t \in p} S_t)|}\\
            &=\sum_{p \in X_{paired}} \sum_{e_j \in \lambda(p)} \frac{w(p)}{|\lambda(p)|}\\
            &=\sum_{p \in X_{paired}} w(p)\\
            &=w(X)
        \end{align}
    \end{proof}

    $\Elements = \{e_{j_1}, e_{j_2}, ..., e_{j_n}\}$ and assume $e_{j_1}$ is covered before or at the same time as $e_{j_2}$ and so on. Based on Lemma \ref{lem_upper} and Equation \ref{equ_1}, we have:

    \begin{align}
        w(X) &= \sum_{e_{j_q}: q \leq n} \frac{\sum_{S_t \in \Gamma(e_{j_q})} w(S_t)}{|Y_{I(e_{j_q})} \cap (\bigcup_{S_t \in \Gamma(e_{j_q})} S_t)|}\\
        &\leq \sum_{e_{j_q}} \frac{L w(X^*)}{|Y_{I(e_{j_q})}|}\\
        &\leq \sum_{e_{j_q}} \frac{L w(X^*)}{n - q + 1} \label{convert_to_num}\\
        &\leq L H_n w(X^*) = O(L \log(n)) w(X^*)
    \end{align}

    The line ~\ref{convert_to_num} is true because, when we are covering $e_{j_q}$ in the iteration $I(e_{j_q})$, there are at least $n - q - 1$ points that are not covered so far which are $\{e_{j_q}, e_{j_{q + 1}}, ..., e_{j_n}\}$.
    
\end{proof}

\subsection{Weighted Faster}

In the above algorithm, at each step, we should check all possible $k$-tuples of sets belonging to all colors. This would have a time complexity of $O(n^k)$. 

In this section we would give an approximation algorithm to give this tuple with minimum $\frac{\sum_i w_i}{|\bigcup_i S_i|}$ value with an approximation ratio of $\frac{e}{e - 1}$ and a time complexity of $O(n \times LP)$ where $LP$ is the time complexity of solving LP.

Let's say we want to find this optimum $k$-tuple. If we know that $|\bigcup_i S_i|$ in this tuple is at least $b$ for a given integer $b$, then it would be sufficient to solve the following LP to find that tuple:

\begin{align}
    \min \sum_{i: S_i \in \mathcal{S}} w_i x_i&\\
    \sum_{j: p_j \in U} y_j &\geq b\\
    \sum_{i: p_j \in S_i} x_i &\geq y_j\\
    \sum_{i: S_i \in c_h} x_i &= 1 \quad \forall h \in \mathcal{C}
\end{align}

Assign a value $x_i$ to each set $S_i \in \mathcal{S}$ and a value $y_j$ to the points $p_j \in U$. Pick a set from each color according to the last constraint of the above LP.

After solving the above LP, I will sample one set from each color according to their probabilities $x_i$. $\square$

{\bf Claim 1}: The result $k$-tuple has an expected length of at least $(1 - \frac{1}{e}) b$.

{\bf Proof}: Let $\epsilon_j$ denote the probability that $p_j$ is not present in the union of these $k$ sets:

\begin{align}
    P(\epsilon_j) &= \prod_{h: h \in \mathcal{C}} (1 - \sum_{i: x_i \in c_h, p_j \in x_i} x_i)\\
    &\leq \prod_{h: c_h \in \mathcal{C}} exp(-\sum_{i: x_i \in c_h, p_j \in x_i} x_i)\\
    &= exp(-\sum_{i: p_j \in x_i} x_i)\\
    &\leq e^{- y_j}
\end{align}

As a result, the probability of covering $y_j$ is at least $1 - \frac{1}{e^{y_j}} \geq (1 - \frac{1}{e})y_j$.

Now we can calculate the expected length of covered points by this tuple.

\begin{align}
    E(covered) &= \sum_{j: p_j \in U} P(y_j \; covered)\\
    &= \sum_{j: p_j \in U} 1 - P(\epsilon_j)\\
    &\geq \sum_j (1 - \frac{1}{e})y_j\\
    &\geq (1 - \frac{1}{e}) b \quad \square
\end{align}

{\bf Claim 2}: The expected cost of sampled $k$-tuple is equal to $opt$. Where $opt$ is the solution to the above LP.

{\bf Proof}: Each set is being picked by the probability of $x_i$. As a result, the expected cost is $\sum_i w_i x_i$ which is equal to the $opt$. $\square$

We will show the cost of a tuple $T$ (sum of weights) with $cost(T)$ and the size of the union of sets in this tuple with $size(T)$.

Back to our algorithm, for every integers $b \leq n$, I should solve the above LP and sample a $k$-tuple $T_b$ using the above randomized rounding. The expected cost of this sampled tuple is equal to optimum cost. As a result, we will check the values $\frac{cost(T_b)}{b}$ for all $b$ to find the minimum value.

After finding the minimum value, for a $b = b^*$, we will use $T_{b^*}$ as my tuple for this greedy step. 

Let's say the tuple $T^*$ is the optimum solution with minimum $\frac{cost(T)}{size(T)}$ value between all tuples. In the expectation, $cost(T_{b^*}) = cost(T^*)$ but $size(T_{b^*}) \geq (1 - \frac{1}{e}) size(T^*)$:

\begin{align}
    \frac{cost(T_{b^*})}{size(T_{b^*})} \leq \frac{e}{e - 1} \frac{cost(T^*)}{size(T^*)} = \frac{e}{e - 1} opt
\end{align}

The running time of above algorithm is $n$ times the time complexity of solving LP (because I'm solving LP for all $b \leq n$).
